# Supplementary material for: kogito: A Commonsense Knowledge Inference Toolkit
Source: arXiv:2211.08451 source file (2023-03-08)
Supplement: Supplementary file 1 [file appendix.tex]

% \begin{figure*}[t]
%     \centering
%     \includegraphics[width=\linewidth]{demo.pdf}
%     \caption{Screenshot from demo app for \kogito{}}% \antoine{Can we make this a PDF instead?}} [done]
%     \label{demo-shot} 
% \end{figure*}
